# Supplementary material for: V-MIND: Building Versatile Monocular Indoor 3D Detector with Diverse 2D Annotations
Source: arXiv:2412.11412 source file (2024-12-16)
Supplement: Supplementary file 1 [file supp_class_stat.tex]

\begin{figure*}[!htb]
    \centering
    \includegraphics[width=0.97\textwidth]{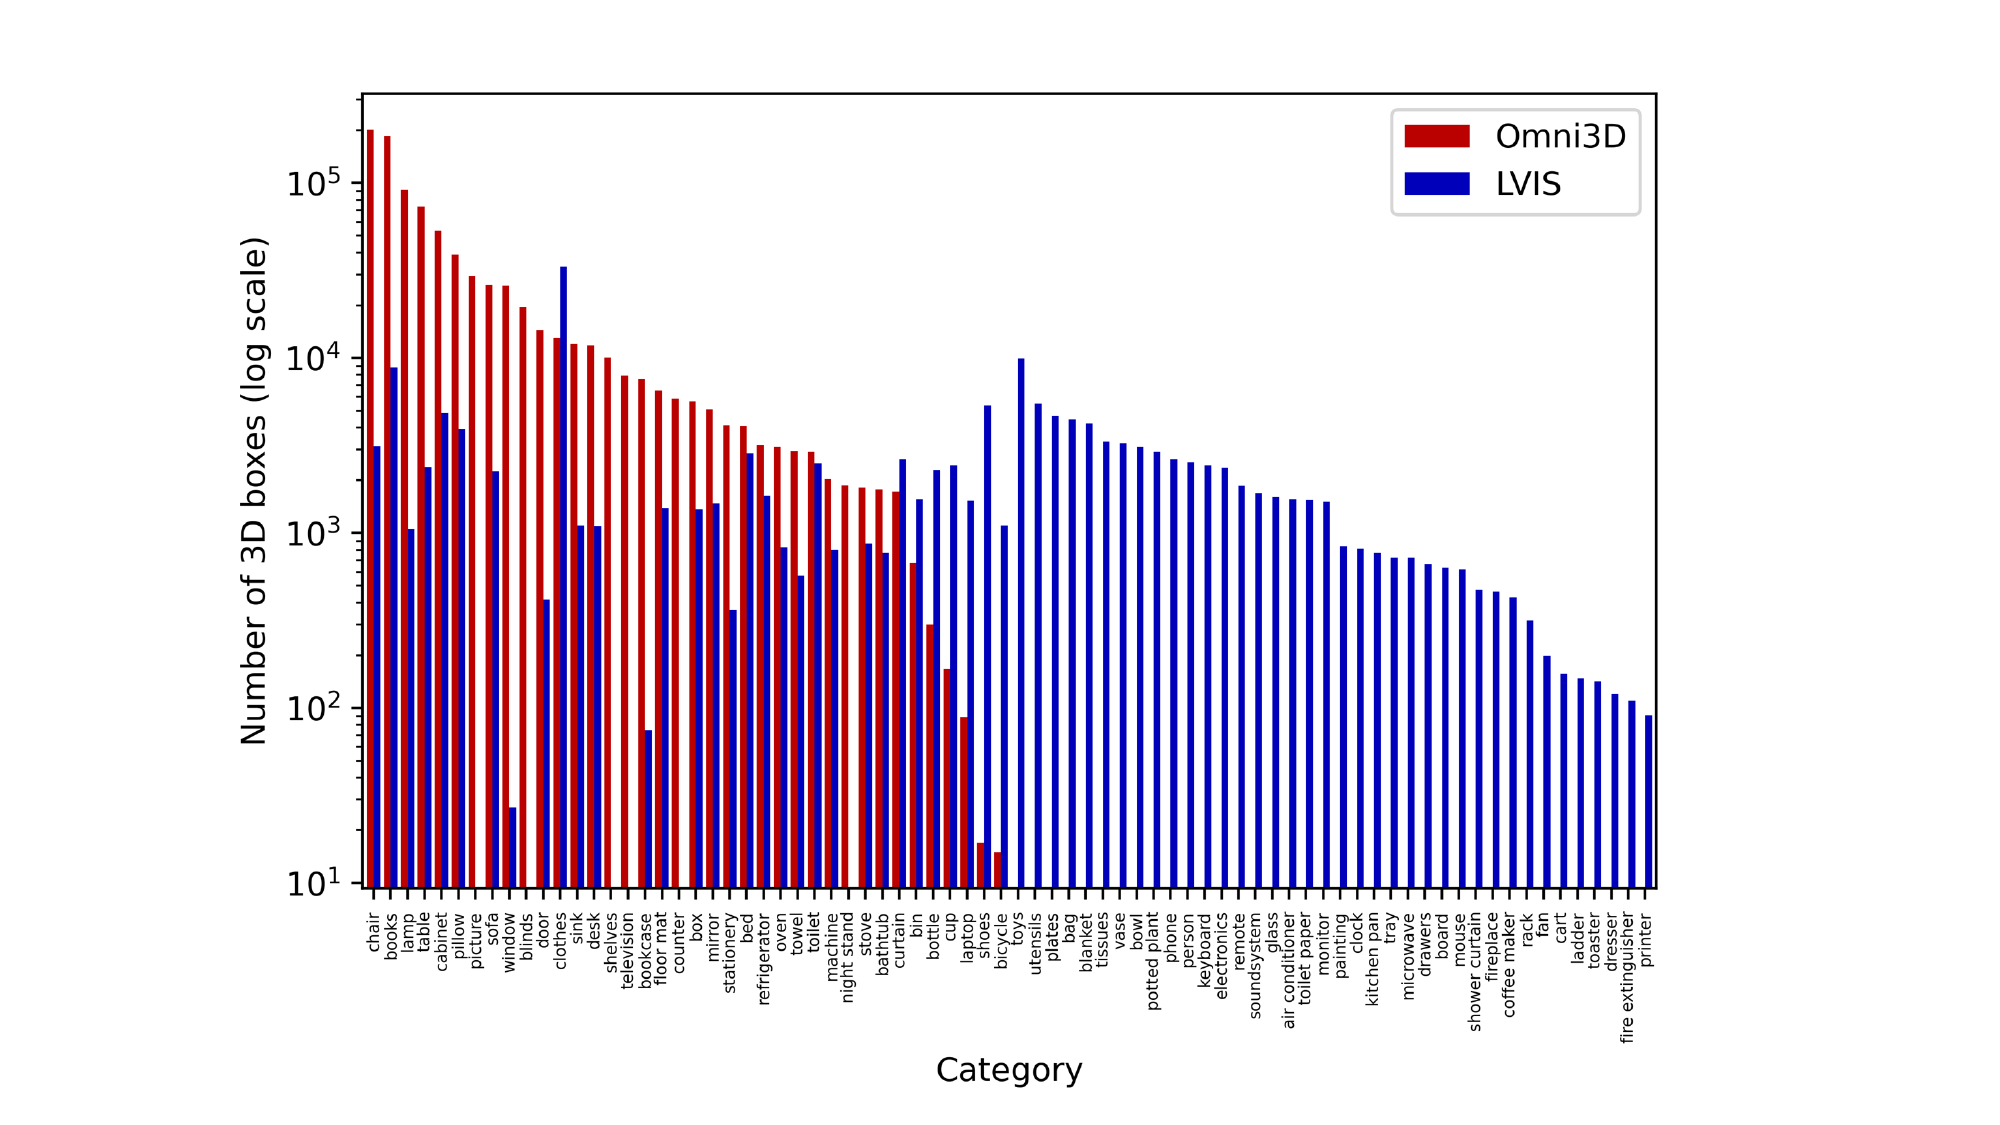}
    \caption{\textbf{Per class training data distribution.} The bar chart presents the number of 3D boxes of the Omni3D~\cite{omni3d} indoor dataset and the lifted LVIS~\cite{gupta2019lvis} data on a logarithmic scale. 
    The original classes, ranging from \textit{chair} to \textit{bicycle}, and the new classes, from \textit{toys} to \textit{printer}, are shown on the x-axis. 
    Our generated data from the LVIS~\cite{gupta2019lvis} dataset spans a wide range of object categories, with a substantial number of 3D pseudo bounding boxes.
    }
    \label{fig:class_stat}
\end{figure*}
