# Supplementary material for: V-MIND: Building Versatile Monocular Indoor 3D Detector with Diverse 2D Annotations
Source: arXiv:2412.11412 source file (2024-12-16)
Supplement: Supplementary file 3 [file supp_qualitative.tex]

\begin{figure*}[h]
    \centering
    \includegraphics[width=0.98\textwidth]{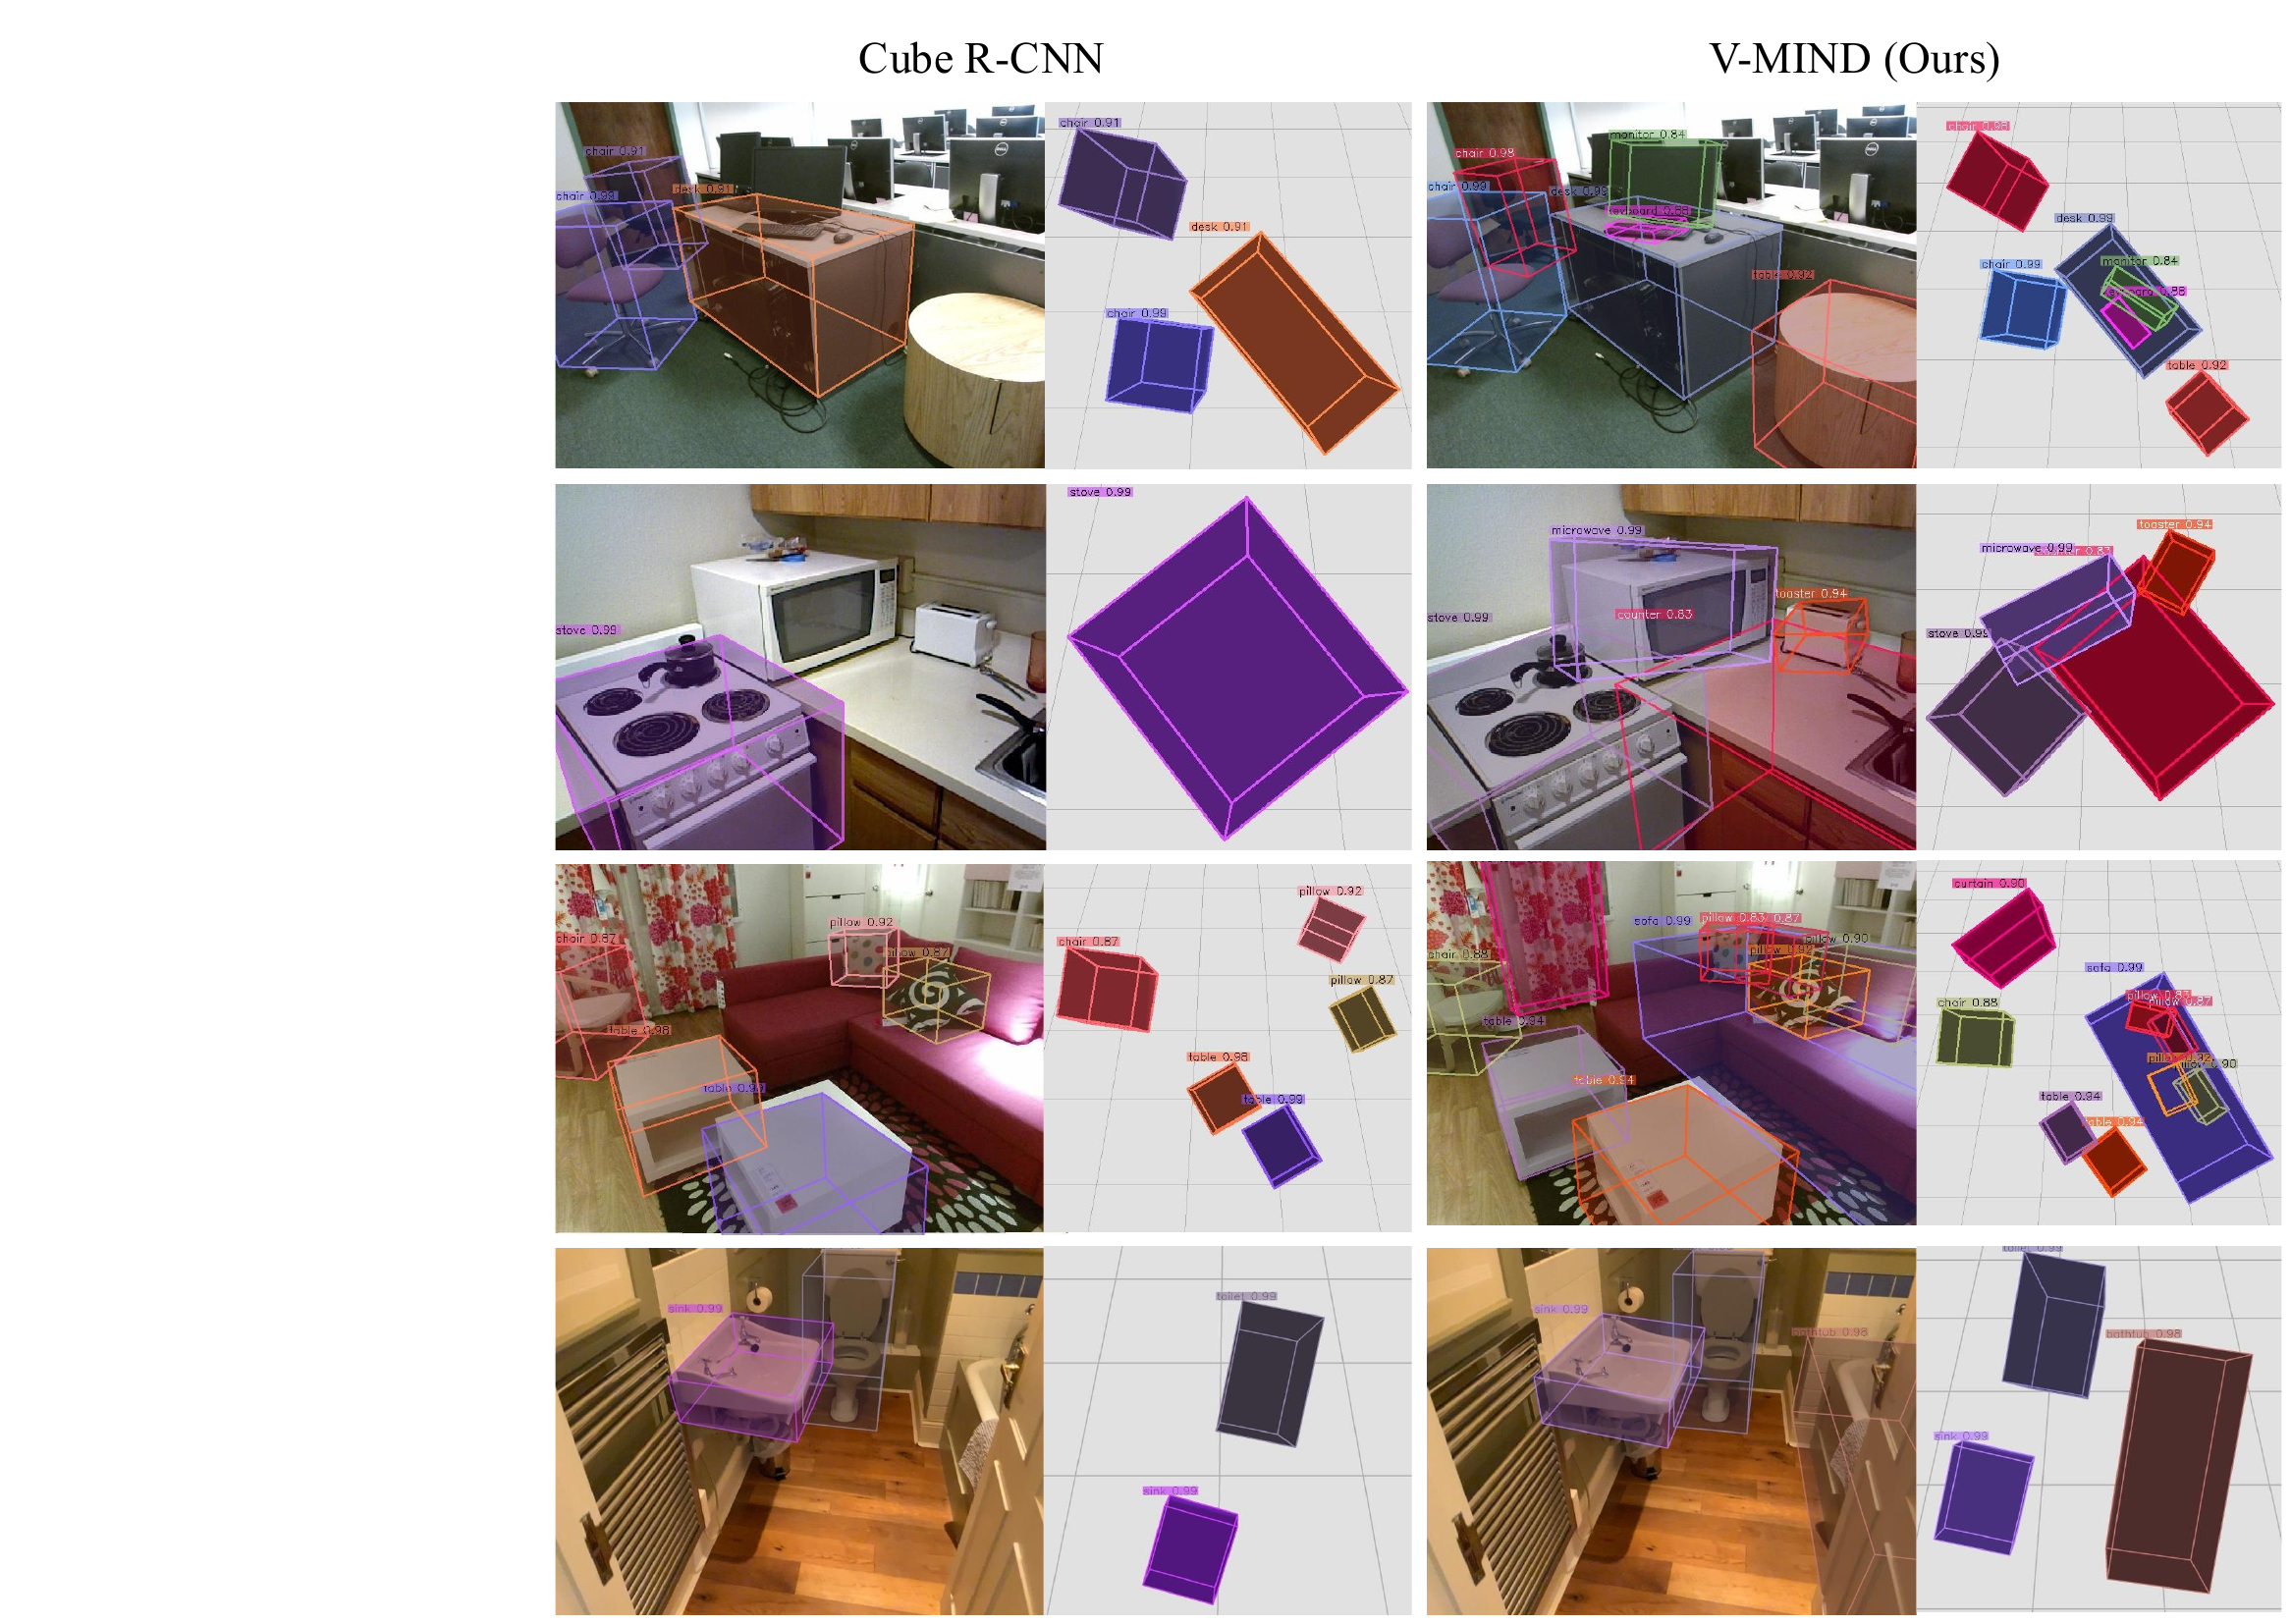}
    \caption{\textbf{Qualitative results of {\ours} and baseline Cube R-CNN.}
    Through our proposed method, {\ours} has the ability to detect a wider range of object classes in 3D.
    For example, the monitor and keyboard in the first row, as well as the microwave and toaster in the second row, are all new classes that are not present in the human-annotated 3D training data. 
    This demonstrates the effectiveness of our proposed method.}
    \label{fig:supp_qualitative}
    
    \vspace*{15pt}
\end{figure*}
