# Supplementary material for: V-MIND: Building Versatile Monocular Indoor 3D Detector with Diverse 2D Annotations
Source: arXiv:2412.11412 source file (2024-12-16)
Supplement: Supplementary file 4 [file supp_filtering_stat.tex]

\begin{table*}[!htb]
% \small
\centering
\caption{
    \textbf{The statistics of the number of pseudo boxes at different stages of the filtering process for the LVIS~\cite{gupta2019lvis} dataset}.
    The negative numbers indicate the \textit{reduction} in the number of pseudo boxes at each filtering stage.
    Since our paper focuses on indoor object detection, the majority of boxes are filtered out during class filtering as they correspond to outdoor categories.
}

\begin{tabular}{l|c|ccc|c}
\toprule
                          &  Original \#boxes &  Class filtering  &  Cube R-CNN filtering~\cite{omni3d}  &  Point filtering  &  Final \#boxes   \\ \midrule
LVIS~\cite{gupta2019lvis} &  790,884   &  -459,840         &  -80,191             &  -87,165         &  163,688       \\
\bottomrule
\end{tabular}

\label{table:filter_stat}
\end{table*}
