# Supplementary material for: V-MIND: Building Versatile Monocular Indoor 3D Detector with Diverse 2D Annotations
Source: arXiv:2412.11412 source file (2024-12-16)
Supplement: Supplementary file 5 [file supp_img_anno_stat.tex]

\begin{table}[!htb]
% \small
\centering
\caption{
    \textbf{The statistics of the training data for each dataset}. 
    We include only the training split of the LVIS~\cite{gupta2019lvis} dataset for our pseudo data generation.
    The ARKitScenes~\cite{dehghan2021arkitscenes} and Hypersim~\cite{hypersim} are multi-view datasets, where many duplicate images and boxes represent the same scenes.
    Additionally, the Hypersim is a synthetic dataset, making it easier to generate large amounts of data but prone to domain gaps.
    In contrast, the data we generate from the 2D LVIS dataset is real-world, diverse, and contains a substantial number of instances.
}
\resizebox{0.47\textwidth}{!}
{
\begin{tabular}{l|rr|rr}
\toprule
\multicolumn{1}{l}{}      & \multicolumn{2}{c}{\#Images}  & \multicolumn{2}{c}{\#Boxes} \\ \midrule
                          &  Train  &  Val   &  Train    &  Val   \\ \midrule
LVIS~\cite{gupta2019lvis} &  48,759 &  -     &  163,688  & -      \\
SUN-RGBD~\cite{SUNRGBD}   &  4,639  &  333   &  18,913   & 1,321  \\
ARKitScenes~\cite{dehghan2021arkitscenes}    &  43,687   & 4,791 &  95,730 & 10,945 \\
Hypersim~\cite{hypersim}  &  48,978 &  6,738 &  674,206  & 75,046 \\
\bottomrule
\end{tabular}
}
\label{table:img_anno_stat}
\end{table}
